# Supplementary material for: Learning-based Compressive Subsampling
Source: arXiv:1510.06188 source file (2016-03-28)
Supplement: Supplementary file 1 [file appendix.tex]

%Here we provide the proof of Theorem \ref{thm:submodular}.  \textbf{[TODO: Edit...currently all copied from Vipul's note]}
%
%\subsection{Proof for the $\ell_{\infty}$-norm}
%
%Sensing matrix is given by:
%$$\textbf{A} = \textbf{PH},$$
%where H is the Hadamard matrix and P is a truncated permutation matrix.\\
%Metric $\textbf{B} = \textbf{A}^T\textbf{A} = \textbf{H}^T\textbf{P}^T\textbf{PH}$.\\
%We would like to minimize $|\textbf{v}_l^T\textbf{Bv}_l - 1|$ for all $l = 1,2,\cdots,M.$\\
%Instead, we try to solve the following problem 
%\begin{equation}
%\underset {\mathbf{B}}\min~ \|\text{diag}(\textbf{V}^T\textbf{BV}) - \textbf{1}_M\|_{\infty} \label{eq:Vipta1}
%\end{equation}
%subject to the conditions $\textbf{B} \geq 0$ and $\text{rank}(\textbf{B}) = r$.
%In our case, the problem can be simplified as
%\begin{eqnarray*}
%\text{diag}(\textbf{V}^T\textbf{BV}) &=& \text{diag}(\textbf{V}^T\textbf{H}^T\textbf{P}^T\textbf{PHV})\\
%&=&\text{diag}({ \mathbf{\tilde V}}^T\mathbf{D \tilde V})
%\end{eqnarray*}
%Here $\mathbf{\tilde V} = \textbf{HV}$ and $\textbf{D} = \textbf{P}^T\textbf{P}$. So, if the number of non-zero entries in truncated permutation matrix $\textbf{P}$ is $r$, then $\textbf{D} = \textbf{P}^T\textbf{P}$ would be a diagonal matrix with only $r$ ones in the diagonal. \\
%
% Let $\mathcal I = \{i|D_{ii} = 1\}$ be a set with $|\mathcal I| = r$. This will ensure that the rank of $\textbf{B}$ is $r$. Also, let $[\tilde{\textbf{v}}_1, \tilde{\textbf{v}}_2,\cdots,\tilde{\textbf{v}}_M]$ be the columns of $\mathbf{\tilde V}$, where $M$ is the number of secants.\\
%Therefore, 
%\begin{equation}
%\mathbf {\tilde v}_j^T\mathbf{D \tilde v}_j = \sum_{i \in \mathcal{I}}\tilde{\mathbf{v}}_{j,i}^2 ~~\forall~ j = [1,2,\cdots,M].
%\end{equation}
%
% The R.H.S. in (2) is $\leq 1$ as we have $\| \tilde{\textbf{v}}_j\|_2 = 1~~\forall~ j = [1,2,\cdots,M].$ 
%As a consequence $$|\mathbf {\tilde v}_j^T\mathbf{D \tilde v}_j - 1| = 1 - \sum_{i \in \mathcal{I}}\tilde{\mathbf{v}}_{j,i}^2.$$
%
% Hence, $\|\text{diag}(\textbf{V}^T\textbf{BV}) - \textbf{1}_M\|_{\infty} = \underset {j=1,\cdots,M} {\max} (1 - \sum_{i \in \mathcal{I}}\tilde{\mathbf{v}}_{j,i}^2),$
%and the problem in (1) can be rewritten as 
%\begin{eqnarray*}
%&~&\underset {|\mathcal I| = r}\min~ \underset {j=1,\cdots,M} {\max} 1 - \sum_{i \in \mathcal{I}}\tilde{\mathbf{v}}_{j,i}^2\\
%&=&\underset {|\mathcal I| = r}\min~ 1 - \underset {j=1,\cdots,M} {\min}\sum_{i \in \mathcal{I}}\tilde{\mathbf{v}}_{j,i}^2\\
%&=&1 - \underset {|\mathcal I| = r}\max~\underset {j=1,\cdots,M} {\min}\sum_{i \in \mathcal{I}}\tilde{\mathbf{v}}_{j,i}^2.
%\end{eqnarray*}
%
% So, the problem we aspire to solve is
%\begin{equation}\label{max-min}
%\underset {|\mathcal I| = r}\max~\left(\underset {j=1,\cdots,M} {\min}\sum_{i \in \mathcal{I}}\tilde{\mathbf{v}}_{ij}^2\right)
%\end{equation} 
%which looks easy to solve (but looks are sometimes deceiving).
%
%\subsection{Proof for the $\ell_1$-norm}
%
%However, if we change our original problem in \eqref{eq:Vipta1} to the following
%\begin{eqnarray}
%\underset {\mathbf{B}}\min~ \|\text{diag}(\textbf{V}^T\textbf{BV}) - \textbf{1}_M\|_{1}\\
%\text{s.t.}~ \textbf{B}\geq 0,~ \text{rank}(\textbf{B}) = r,\nonumber
%\end{eqnarray}
%which suggests that we are interested in taking only the average of penalties and hence not giving more weight to the outliers, then, the problem for our case boils out to
%$$\underset {|\mathcal I| = r}\max~\left(\sum_{{{i \in \mathcal{I}},j=1}}^M\tilde{\mathbf{v}}_{j,i}^2\right),$$
%which also looks easy to solve (looks are not always deceiving). We just have to sum the entries of $\mathbf{\tilde V}$ row-wise and find the indices of maximum $r$ values. This will give us the set $\mathcal I$, which can be used to form the matrix $\textbf{D}$.   
%
%\subsection{Proof for the $\ell_2$-norm}
%
%Sensing matrix is given by:
%$$\textbf{A} = \textbf{PH},$$
%where H is the Hadamard matrix and P is a truncated permutation matrix.\\
%Metric $\textbf{B} = \textbf{A}^T\textbf{A} = \textbf{H}^T\textbf{P}^T\textbf{PH}$.\\
%We would like to minimize $|\textbf{v}_l^T\textbf{Bv}_l - 1|$ for all $l = 1,2,\cdots,M.$\\
%Therefore, we try to solve the following problem, which minimizes the average of squares of penalties 
%\begin{equation}
%\underset {\mathbf{B}}\min~ \|\text{diag}(\textbf{V}^T\textbf{BV}) - \textbf{1}_M\|_2^2
%\end{equation}
%subject to the conditions $\textbf{B} \geq 0$ and $\text{rank}(\textbf{B}) = r$.
%In our case, the problem can be simplified as
%\begin{eqnarray*}
%\text{diag}(\textbf{V}^T\textbf{BV}) &=& \text{diag}(\textbf{V}^T\textbf{H}^T\textbf{P}^T\textbf{PHV})\\
%&=&\text{diag}({ \mathbf{\tilde V}}^T\mathbf{D \tilde V})
%\end{eqnarray*}
%Here $\mathbf{\tilde V} = \textbf{HV}$ and $\textbf{D} = \textbf{P}^T\textbf{P}$. So, if the number of non-zero entries in truncated permutation matrix $\textbf{P}$ is $r$, then $\textbf{D} = \textbf{P}^T\textbf{P}$ would be a diagonal matrix with only $r$ ones in the diagonal. \\
%
% Let $\mathcal I = \{i|D_{ii} = 1\}$ be a set with $|\mathcal I| = r$. This will ensure that the rank of $\textbf{B}$ is $r$. Also, let $[\tilde{\textbf{v}}_1, \tilde{\textbf{v}}_2,\cdots,\tilde{\textbf{v}}_M]$ be the columns of $\mathbf{\tilde V}$, where $M$ is the number of secants.\\
%Therefore, 
%\begin{equation}
%\mathbf {\tilde v}_j^T\mathbf{D \tilde v}_j = \sum_{i \in \mathcal{I}}\tilde{v}_{ij}^2 ~~\forall~ j = [1,2,\cdots,M]. \label{eq:Vipta2}
%\end{equation}
%
% The R.H.S. in \eqref{eq:Vipta2} is $\leq 1$ as we have $\| \tilde{\textbf{v}}_j\|_2 = 1~~\forall~ j = [1,2,\cdots,M].$ 
%As a consequence $$|\mathbf {\tilde v}_j^T\mathbf{D \tilde v}_j - 1| = 1 - \sum_{i \in \mathcal{I}}\tilde{v}_{ij}^2.$$
%
% Hence, $\|\text{diag}(\textbf{V}^T\textbf{BV}) - \textbf{1}_M\|_2 = \sum_{j=1}^M(1 - \sum_{i \in \mathcal{I}}\tilde{v}_{ij}^2)^2,$
%and the problem in (1) can be rewritten as 
%\begin{eqnarray*}
%&~&\underset {|\mathcal I| = r}\min~ \sum_{j=1}^M(1 - \sum_{i \in \mathcal{I}}\tilde{v}_{ij}^2)^2\\
%&=&\underset {|\mathcal I| = r}\max~ -\sum_{j=1}^M(1 - \sum_{i \in \mathcal{I}}\tilde{v}_{ij}^2)^2
%\end{eqnarray*}
%
%\textbf{Proof of Submodularity:}
%
%Show that if for all $j$ we have $\sum\limits_i \tilde{v}_{ij}^2=1$ and $\tilde{v}_{ij}^2\ge0$ then the function
%$$f(I)=-\sum\limits_j(1-\sum\limits_{i\in I}\tilde{v}_{ij}^2)^2$$
%with $I\subseteq \{1\dots n\}=\Omega$ is submodular.
%
%It is well known that submodularity is preserved under taking nonnegative linear combinations, so it will be enough to show that the function
%
%$$g(I)=-(1-\sum\limits_{i\in I}\tilde{v}_{ij}^2)^2$$
%for all $j\in\{1\dots m\}$ and $I\subseteq \Omega$ is submodular.
%
%By the definition of submodular functions, $g(I)$ is submodular iff for every $I \subseteq \Omega$ and $y,z\in \Omega\setminus I$ we have that $$g(I\cup \{y\})+g(I\cup \{z\})\geq g(I\cup \{y,z\})+g(I)$$ 
%
%Let's rename for simplicity $\sum\limits_{i\in I}\tilde{v}_{ij}^2=A$, $\tilde{v}_{yj}^2=Y$ and $\tilde{v}_{zj}^2=Z$. Then, it suffices to show that the following claim holds.
%
%For any $0\le A,Y,Z\le 1$ we have 
%\begin{eqnarray*}
%(1-A-Y)^2+(1-A-Z)^2 &\leq& (1-A-Y-Z)^2 + (1-A)^2.\\
%\end{eqnarray*}
%Also,
%\begin{eqnarray*}
%&~&(1-A-Y)^2+(1-A-Z)^2\\
%&=&(1-A)^2 - 2(1-A)Y+Y^2+ (1-A)^2 - 2(1-A)Z+Z^2\\
%&=&(1-A)^2+Y^2+Z^2 - 2(1-A)Y- 2(1-A)Z +2YZ -2YZ + (1-A)^2 \\
%&=&(1-A-Y-Z)^2  -2YZ+ (1-A)^2 \\ 
%&\leqslant& (1-A-Y-Z)^2 + (1-A)^2  
%\end{eqnarray*}
%
%Note that the only condition we used was $Y,Z \geqslant 0$
%
